# Supplementary material for: ProtoBandit: Efficient Prototype Selection via Multi-Armed Bandits
Source: arXiv:2210.01860 source file (2023-08-23)
Supplement: Supplementary file 1 [file appendix_survey.tex]

\section{Brief Background on Approximate Greedy Search and Multi-armed Bandits}

\subsection{Approximate Greedy Search}
\citet{bib:Minoux:1978} introduced an \textsc{Accelerated Greedy} algorithm that employs an intelligent search through the set, and it requires a number of function evaluations that is minimum among all greedy algorithms. 
The author showed that if the solution of classical greedy algorithm is unique, then the solution found by \textsc{Accelerated Greedy} will coincide.
Therefore, like greedy, the algorithm offers $(1-\exp(-1))$ approximation ratio but improves the running time. \citet{bib:Wei+IB:2014} proposed computationally cheaper and faster algorithm \textsc{MultGreed} that relaxes the greedy searching criteria of \textsc{Accelerated Greedy} to give an approximation ratio $(1-\exp(-\beta)$, for an input parameter $\beta \in (0, 1)$. \citet{bib:Badanidiyuru+V:2014} presented another fast approximate greedy search algorithm that offers $(1-\exp(-1)\epsilon)$, and by following the naming convention adopted by ~\citet{bib:Mirzasoleiman+BKVK:2015} let us call this \textsc{ThresholdGreedy}.  
Later, \citet{bib:Mirzasoleiman+BKVK:2015} proposed an algorithm \textsc{Stochastic-Greedy} that employs random-sampling to quickly search through the set of points, and uses the lazy-evaluation method of \textsc{Accelerated Greedy}. Therefore, besides offering $(1-\exp(-1)\epsilon)$ approximation, \textsc{Stochastic-Greedy} was shown to be more empirically efficient than \textsc{ThresholdGreedy}. As our objective is to build a  prototype selection algorithm that can operate at arbitrarily large scale, we build the mechanism on \textsc{Stochastic-Greedy} algorithm. One shortcoming of  \textsc{Stochastic-Greedy} is that it needs the exact value of the function, which might be quite computationally expensive. We mitigate this issue via PAC selection through sampling using Multi-Armed Bandits (MAB)~\citep{bib:Berry+F:1985} set up that we introduce next.

\subsection{ Multi Armed bandits and the Pure Exploration Problem} 

Multi-Armed Bandits~\citep{bib:Berry+F:1985} is a popular abstraction of sequential decision making under the uncertainty. An \emph{arm} of a bandit represents a decision, while \emph{pull} of an arm represents taking decision corresponding to that arm. Further, we assume each arm has an probability distribution associated with it, and when pulled, a real-valued reward is generated in i.i.d. fashion from the underlying probability-distribution. This probability distribution is called reward distribution of that particular arm, and is unknown to the experimenter.
For simplicity, we assume the reward-distribution for each arm is supported on the interval $[0, 1]$. Under the scenario like A/B testing it is an interesting problem to identify the best arm incurring  minimal number of total  samples. To put formally, we assume $\mathcal{A}$ be the given set of $n$ arms with $\mu_a$ being the expected mean reward of arm $a \in \mathcal{A}$. For simplicity, we assume, $\mu_{a_1} \geq \mu_{a_2} \geq \cdots \mu_{a_n}\geq 0$. As the reward distribution of the arms are not known, it can be trivially shown that there is no algorithm that incurs a finite number of samples to identify the arm with the highest expected reward with certainty. Hence, we seek for an approximate solution. 
For simplicity, we inherit some notations from  ~\citet{bib:RoyChaudhuri+K:2019}. For a given tolerance $\epsilon \in [0, 1]$, we call an arm $a$ to be \emph{$(\epsilon, m)$-optimal} if $\mu_a \geq \mu_{a_m}$. We define set of all $(\epsilon, m)$-optimal arms by $\mathcal{TOP}_m(\epsilon) \defeq \{a: \mu_a \geq \mu_{a_m}\}$. Now, we re-state the following problem from ~\citep{bib:RoyChaudhuri+K:2019}:

\begin{definition}[$(k,m,n)$ \textbf{Problem}]
An instance of the $(k, m, n)$ problem
is of the form $(\mathcal{A}, n, m, k, \epsilon, \delta)$, where $\mathcal{A}$ is a set of arms
with $|\mathcal{A}| = n \geq 2$; $m \in \{1, 2, \cdots, n-1\}$; $k \in \{1, \cdots, m\}$;
tolerance $\epsilon \in (0, 1]$; and mistake probability $\delta \in (0, 1]$. An
algorithm $L$ is said to solve $(k, m, n)$ if for every instance
of $(k, m, n)$, it terminates with probability 1, and returns $k$
distinct $(\epsilon, m)$-optimal arms with probability at least $1-\delta$.
\end{definition}

This $(k,m,n)$ problem is interesting as it generalises a whole spectrum of problems. For $k= m = 1$, the problem reduces to identifying an  $(\epsilon, 1)$-optimal, which is the best-arm identification problem.
\citet{bib:Even-Dar+MM:2002} presented an in-depth study on the best-arm identification problem, and an algorithm \textsc{Median Elimination} that solves the problem using sample complexity $O\left(\frac{n}{\epsilon^2}\log\frac{1}{\delta}\right)$. \citet{bib:Mannor+T:2004} showed that number of samples incurred by \textsc{Median Elimination} lies within a constant factor of the lower bound. The idea of the algorithm lies in pruning out the suboptimal arms using a small number of samples, and assigning further pulls to the arms that harder to distinguish from the optimal arm. However, due the large value of the preceding constant the algorithm incurs more sample than naive elimination method if the number of arms are less than $10^5$. Recently, ~\citet{bib:Hassidim+KS:2020} have proposed an algorithm \textsc{Approximate Best Arm} (\textsc{Aba}) that uses Aggressive Elimination ~\citep{bib:Hassidim+KS:2020} for a well-balanced exploration strategy to reduce the number of arms to $n^{3/4}/2$, such that the optimal arm belongs to the output set with high-probability. Then, it uses Naive Elimination strategy to output an $(\epsilon ,1)$-optimal arm. This combined strategy adapted by ABA helps it to incur a much smaller number of samples. The authors show that for $\delta <0.05$, for any $n >0$, and $\epsilon \in (0, 1)$ the number of samples incurred by ABA is at least 300 times smaller as compared to \textsc{Median Elimination}. \citet{bib:Hassidim+KS:2020} also present some modifications of ABA like \textsc{Simple Approximate Best Arm} (\textsc{Saba}), and  Approximate Best Arm Likelihood Estimation (\textsc{Abaleh}) that we shall compare in the experiments presented in Section~\ref{sec:experiment}.
% As one of the core-contribution, ~\citet{bib:Hassidim+KS:2020} proposes an algorithm Aggressive Elimination that uses a well-balanced exploration strategy to reduce the number of arms to $n^{3/4}/2$, such that the optimal arm belongs to the output set with high-probability. Once 
% Specifically, ~\citet{bib:Hassidim+KS:2020} breaks down the problem for depending on the relative largeness of $n$, and $\delta$, and proposes a solution for each of the cases. 

It is important to note that the number of samples incurred by \textsc{Median Elimination}~\citep{bib:Even-Dar+MM:2002}  ABA~\citep{bib:Hassidim+KS:2020} are problem-independent; that is the number of samples incurred is independent of mean of the arms. 
% Therefore, such sample-complexity of these algorithms are not affected even if the mean of the arms are indistinguishable or very close to each other. 
However, in practice, it is common to handle set arms whose mean are not very close to each other, and hence it is more efficient to use algorithms like \textsc{LUCB}-$k$-$m$~\citep{bib:RoyChaudhuri+K:2019} (for $k = m =1$), 
\textsc{lil'UCB} etc.\ that take advantage of the difference between mean of the arms. \textsc{LUCB}-k-m can be made even more sample-efficient by adapting a KL-divergence based confidence-bound as done in \textsc{KL-LUCB}~\citep{bib:Kaufmann+K:2013}. We compare these algorithms in Section~\ref{sec:experiment}.
